# Supplementary material for: Assessing the Effects of Orbital Relaxation and the Coherent-State Transformation in Quantum Electrodynamics Density Functional and Coupled-Cluster Theories
Source: arXiv:2303.10821 ancillary file (2023-05-18)
Supplement: Supplementary file 1 [file cqed_eom_ee_ccsd_si.pdf]

# Supporting Information for: Assessing the Effects of Orbital Relaxation and the Coherent-State Transformation in Quantum Electrodynamics Density Functional and Coupled-Cluster Theories


Marcus D. Liebenthal, Nam Vu, and A. Eugene DePrince III*

*Department of Chemistry and Biochemistry, Florida State University, Tallahassee, FL 32306-4390*

E-mail: adeprince@fsu.edu

**Table S1: Ground-state energies ($E_\mathrm{h}$) from relaxed QED-CCSD-1 and absolute energy errors ($10^{-3}$ $E_\mathrm{h}$) from unrelaxed QED-CCSD-1, as well as from relaxed and unrelaxed QED-CCSD-1 calculations that ignore $u_0$. Also provided are $u_0$ values from relaxed and unrelaxed QED-CCSD-1 calculations. All calculations consider $\lambda = 0.1$ atomic units, and the cavity mode is polarized either along the molecular axis or perpendicular to it, as described in the main text.**

| | | | | error | error w/o $u_0$ | | $u_0$ | |
|---|---|---|---|---|---|---|---|---|
| system | $\omega_\mathrm{cav}$ | resonance | relaxed | unrelaxed | relaxed | unrelaxed | relaxed | unrelaxed |
| $H_2$ | 0.466751 | $1^1\mathrm{B}_{1\mathrm{u}}$ | $-1.163485$ | 0.000000 | 0.000000 | 0.000000 | 0.000000 | 0.000000 |
| $H_2$ | 1.522218 | $1^1\mathrm{B}_{2\mathrm{u}}$ | $-1.163222$ | 0.000000 | 0.000000 | 0.000000 | 0.000000 | 0.000000 |
| HF | 0.531916 | $2^1\mathrm{A}_1$ | $-100.288128$ | 0.074971 | 0.011819 | 2.949808 | 0.004067 | -0.074734 |
| HF | 0.375022 | $1^1\mathrm{B}_1$ | $-100.287676$ | 0.060050 | 0.000000 | 0.060051 | 0.000000 | 0.000000 |
| LiF | 0.308401 | $3^1\mathrm{A}_1$ | $-107.222193$ | 0.456170 | 0.029418 | 30.799100 | 0.008246 | -0.320050 |
| LiF | 0.232119 | $1^1\mathrm{B}_1$ | $-107.220994$ | 0.145191 | 0.000000 | 0.145191 | 0.000000 | 0.000000 |

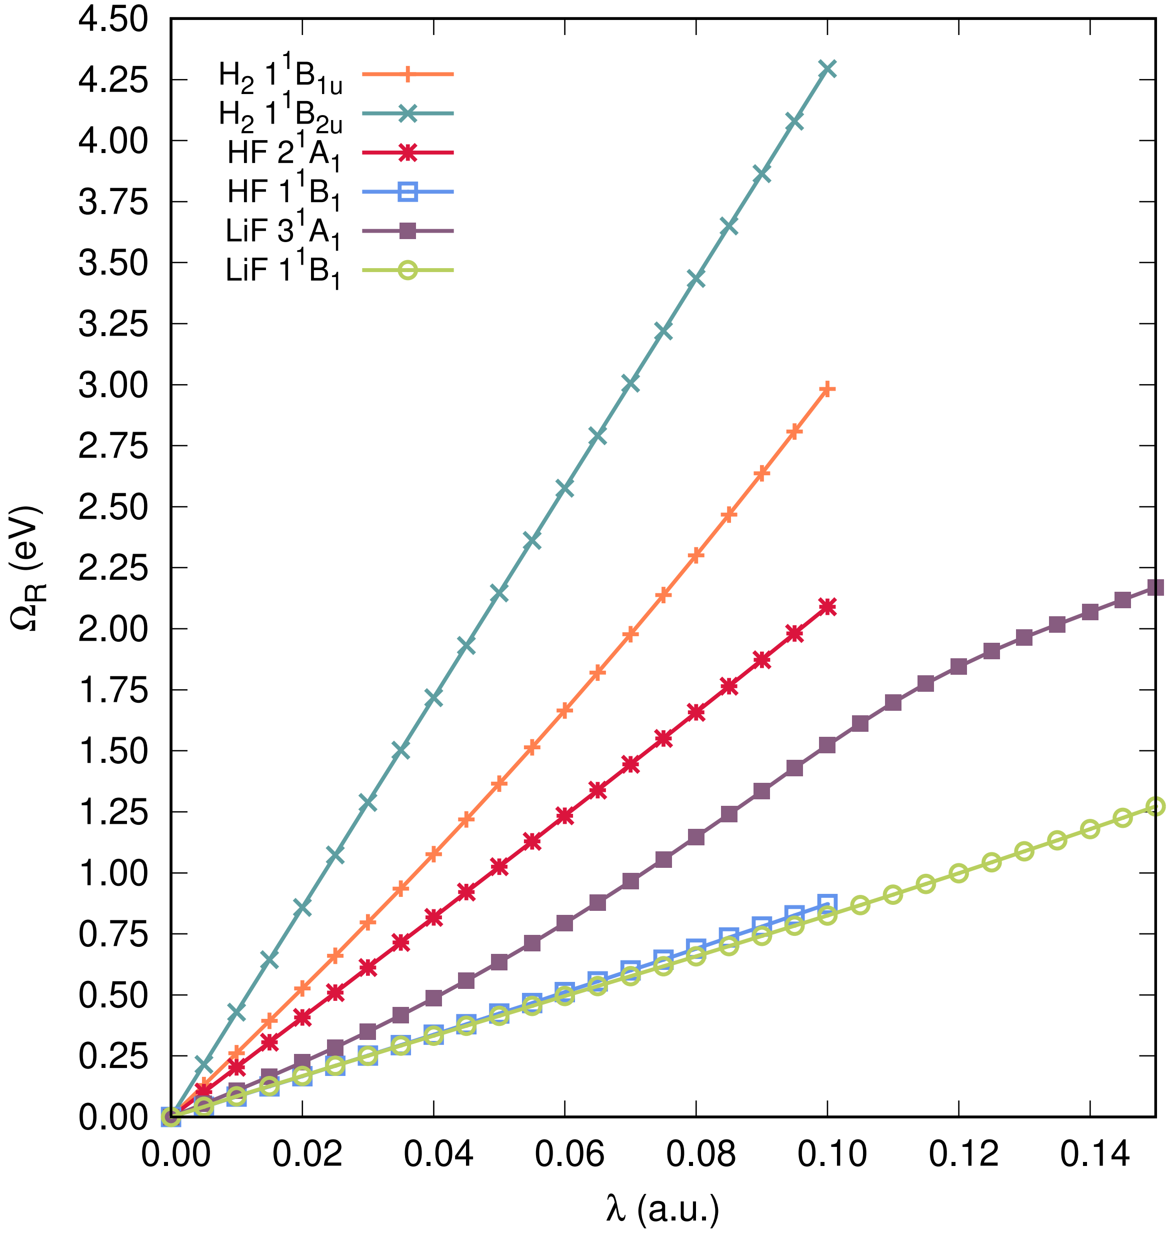


Figure S1: Rabi splittings from relaxed QED-EOM-CCSD-1 as a function of the coupling strength, $\lambda$; details regarding the relative orientation of the cavity mode polarization and the molecular axis can be found in the main text.

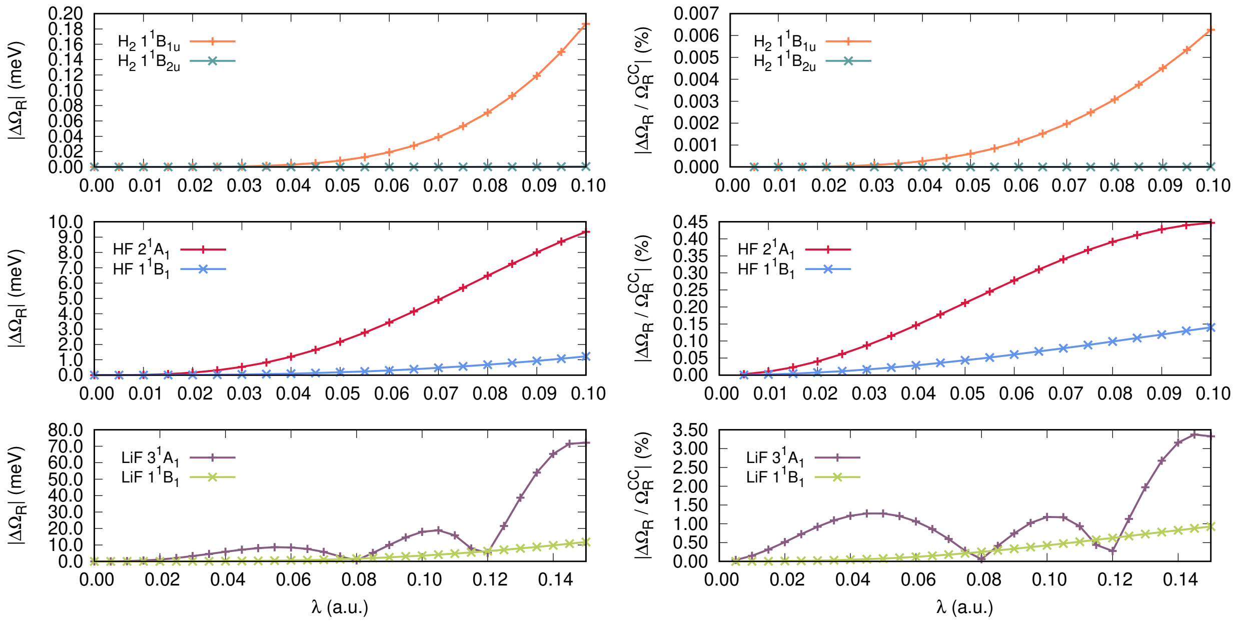


Figure S2: The left column plots the absolute energy differences in Rabi splittings obtained from relaxed and unrelaxed QED-EOM-CCSD-1 as a function of the coupling strength, $\lambda$, for $H_2$, HF, and LiF. The right column plots the same quantities, represented as a percentage. Details regarding the relative orientation of the cavity mode polarization and the molecular axis can be found in the main text.
